# Supplementary material for: Fundamental limits of free-space microwave-to-optical frequency conversion efficiency using Rydberg atoms
Source: arXiv:2411.13160 source file (2024-11-20)
Supplement: Supplementary file 1 [file SM.pdf]

# Supplemental Material for "Fundamental limits of free-space microwave-to-optical frequency conversion efficiency using Rydberg atoms"

Ya-Nan Lv,[1,2,3] Yan-Lei Zhang,[1,2,4,*] Xu-Bo Zou,[1,2,4] Guang-Can Guo,[1,2,4] Shui-Ming Hu,[3] and Chang-Ling Zou[1,2,4,†]

[1]*CAS Key Laboratory of Quantum Information, University of Science and Technology of China, Hefei, Anhui 230026, P. R. China*
[2]*Anhui Province Key Laboratory of Quantum Network, University of Science and Technology of China, Hefei 230026, P. R. China*
[3]*Department of Chemical Physics, University of Science and Technology of China, Hefei 230026, China*
[4]*CAS Center for Excellence in Quantum Information and Quantum Physics, University of Science and Technology of China, Hefei 230026, China*

## CONTENTS

I. Simplified model for Multi-wave mixing S1
A. Four-wave mixing S1
B. Six-wave mixing S1

II. Microwave coupling S2
A. Super-atom coupled to a single microwave channel S2
B. Super-atom coupled to multiple channels S3

III. Optical coupling S3
A. The spin-wave mode S3
B. The evolution of the system S4
C. The mean optical depth $\overline{OD}$ S5

IV. Effective Conversion Hamiltonian S6

V. Method of slicing S6

References S7

## I. SIMPLIFIED MODEL FOR MULTI-WAVE MIXING

This section explains the simplified models for four-wave and six-wave mixing processes, as depicted in Fig. 1b of the main text.

### A. Four-wave mixing

As shown in Fig. 1 is the schematic of the simplified Raman transition for microwave input, which stimulates the transition directly from $|g\rangle$ to $|r\rangle$. For the system of four-wave mixing, the Hamiltonian is given by

$$H = \Delta|r'\rangle\langle r'| + (\Omega|g\rangle\langle r'| + \Omega_{\mathrm{m}}|r'\rangle\langle r| + h.c.). \quad (S.1)$$

Here, $\Delta \gg \Omega, \gamma_{r'}$. For large detuning, we have $\rho_{\mathrm{r'r'}} \approx 0$, and $\rho_{\mathrm{gr'}}, \rho_{\mathrm{r'r}}$ are at their steady states:

$$\rho_{\mathrm{gr'}} \simeq \frac{\Omega}{-\Delta}\rho_{gg} + \frac{\Omega_{\mathrm{m}}}{-\Delta}\rho_{\mathrm{gr}},$$
$$\rho_{\mathrm{r'r}} \simeq \frac{\Omega}{-\Delta}\rho_{\mathrm{gr}} + \frac{\Omega_{\mathrm{m}}}{-\Delta}\rho_{\mathrm{rr}}. \quad (S.2)$$

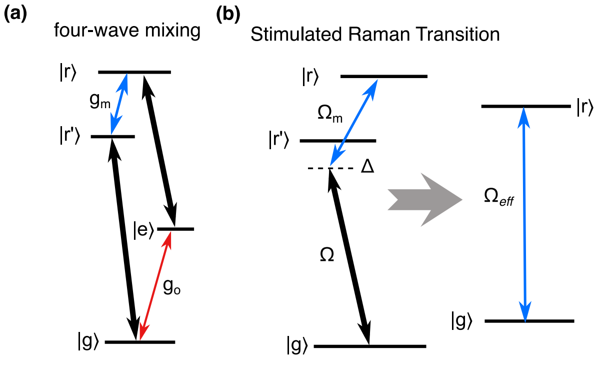


**Supplemental Figure** 1. The schematic of the stimulated Raman transitions for the microwave input in a four-wave mixing model.

Substituting the steady results of $\rho_{\mathrm{gr'}}, \rho_{\mathrm{r'r}}$ into the differential equation for $\rho_{gr}$, we can obtain

$$\frac{\mathrm{d}\rho_{\mathrm{gr}}}{\mathrm{d}t} = -i\Omega\rho_{\mathrm{r'r}} + i\Omega_{\mathrm{m}}\rho_{\mathrm{gr'}} - \frac{\gamma_r}{2}\rho_{\mathrm{gr}}$$
$$\simeq -i\Omega_{\mathrm{eff}}(\rho_{\mathrm{gg}} - \rho_{\mathrm{rr}}) + [i(\frac{\Omega^2}{\Delta} - \frac{\Omega_{\mathrm{m}}^2}{\Delta}) - \frac{\gamma}{2}]\rho_{\mathrm{gr}}, \quad (S.3)$$

Where $\Omega_{\mathrm{eff}} = \Omega\Omega_{\mathrm{m}}/\Delta$ is the effective Rabi frequency for the four-wave mixing process.

### B. Six-wave mixing

In Fig. 2, the model for the six-wave mixing system is illustrated. The Hamiltonian is given by

$$H = \Delta_1|e'\rangle\langle e'| + \Delta_2|r''\rangle\langle r''| + \Delta_3|r'\rangle\langle r'| + \big(\Omega_1|g\rangle\langle e'| + \Omega_2|e'\rangle\langle r''| + \Omega_3|r'\rangle\langle r''| + \Omega_{\mathrm{m}}|r'\rangle\langle r| + h.c.\big). \quad (S.4)$$

Here $\Delta_1, \Delta_2, \Delta_3 \gg \Omega_1, \Omega_2, \Omega_3, \Omega_{\mathrm{m}}, \gamma_{\mathrm{e'}}, \gamma_{\mathrm{r''}}, \gamma_{\mathrm{r'}}$. Thus we can assume that $\rho_{ii} \approx 0$ for intermediate state $i \in [e', r'', r']$, and $\rho_{ij}$ ($i, j \in [g, e', r'', r', r], ij \neq gg, rr, gr, rg$) are at their steady states. Substituting these steady results into the differential equation for $\rho_{gr}$, we can obtain

$$\frac{\mathrm{d}\rho_{\mathrm{gr}}}{\mathrm{d}t} \simeq -i\Omega_{\mathrm{eff}}(\rho_{gg} - \rho_{rr}), \quad (S.5)$$

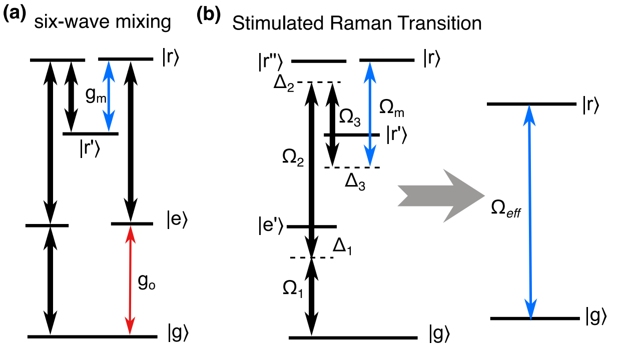


**Supplemental Figure** 2. The schematic of the stimulated Raman transitions for the microwave input in a six-wave mixing model.

where $\Omega_{\mathrm{eff}} = \Omega_1\Omega_2\Omega_3\Omega_{\mathrm{m}}/(\Delta_1\Delta_2\Delta_3)$ is the effective Rabi frequency for the six-wave mixing process.

These simplified models provide valuable insights into the dynamics of four-wave and six-wave mixing processes in multi-level atomic systems.

## II. MICROWAVE COUPLING

### A. Super-atom coupled to a single microwave channel

The excitation of the super-atom excitation $S$, as well as the input-output theory for the free-space microwave coupling with the super-atom, requires the understanding of its coupling to a continuum. Such a continuum could be the three-dimensional vacuum modes in free-space or the free-space propagation Gaussian beam mode. We first consider the simplest model, with the super-atom coupled to a one-dimensional continuum, i.e., a single microwave channel, as

$$H = \omega_s S^\dagger S + \sum_k [\omega_k b_k^\dagger b_k + g_k b_k^\dagger S + g_k^* b_k S^\dagger]. \tag{S.6}$$

Here, the continuum of microwave modes are described by the variable $k$, which corresponds to the wave-vector of a wave. $b_k$ describes the bosonic annihilation operator of the continuum mode, $\omega_k$ is its frequency that determined by the dispersion relationship of the continuum, and $g_k$ is the coupling strength between the super-atom with the continuum mode. The coupling strength could be solved by applying the box quantization of the continuum mode, and the $g_k$ is $\sqrt{N}$ times as large as that of the single atom due to the collective enhancement effect. Consequently, the evolution of operators $S$ and $b_k$ follow

$$\frac{\mathrm{d}b_k}{\mathrm{d}t} = i[H, b_k] = -i\omega_k b_k - ig_k S, \tag{S.7}$$

$$\frac{\mathrm{d}S}{\mathrm{d}t} = i[H, S] \simeq -i\omega_s S - i\sum_k g_k b_k, \tag{S.8}$$

where the Holstein-Primakoff approximation $[S, S^\dagger] \simeq 1$ is applied for the super-atom excitation $S$. Introducing the transformation

$$b_k = e^{-i\omega_k t} f_k(t), \tag{S.9}$$

we obtain

$$\frac{\mathrm{d}f_k(t)}{\mathrm{d}t} = -ig_k e^{i\omega t} S. \tag{S.10}$$

Then, we can get the formal solution of $f(t)$ as

$$f_k(t) = f_k(t_0) + \int_{t_0}^{t} \left[-ig_k e^{i\omega_k t'} S(t')\right] \mathrm{d}t', \tag{S.11}$$

and obtain the solution of $b_k$ as

$$b_k = e^{-i\omega_k(t-t_0)} b_{k,in} - ig_k \int_{t_0}^{t} e^{i\omega_k(t'-t)} S(t')\mathrm{d}t', \tag{S.12}$$

where $b_{k,in} = e^{-i\omega_k t_0} f_k(t_0)$. Substituting the solution of $b_k$ into the evolution equation of $S$, we can obtain

$$\frac{\mathrm{d}S}{\mathrm{d}t} = -i\omega_s S - i\int_0^\infty \rho_k g_k \Big[e^{-i\omega_k(t-t_0)} b_{k,in} - ig_k \int_{t_0}^{t} e^{i\omega_k(t'-t)} S(t')\mathrm{d}t'\Big]\mathrm{d}k, \tag{S.13}$$

where the sum of microwave modes is replaced by the integral $\sum_{k=0}^{\infty} \to \int_0^\infty \rho_k \mathrm{d}k$, with $\rho_k$ denoting the mode density of a one-dimensional microwave field. Since only one direction of the propagating microwave field is considered, the integral of $k$ ranges from 0 to infinity.

Introducing the input field operator

$$b_{in}'(t) = \frac{1}{2\pi}\int_{-\infty}^{\infty} e^{-i\omega(t-t_0)} b_{\omega,in}\mathrm{d}\omega, \tag{S.14}$$

the dynamics of $S$ follow

$$\frac{\mathrm{d}S}{\mathrm{d}t} = -i\omega_s S - ig_\omega\rho_\omega 2\pi b_{in}' - \int_{-\infty}^{\infty} \rho_\omega g_\omega^2 \int_{t_0}^{t} e^{-i\omega(t-t')} S(t')\mathrm{d}t'\mathrm{d}\omega. \tag{S.15}$$

By exchanging the order of integration of time and frequency and using the relations

$$\int_{-\infty}^{\infty} e^{-i\omega(t-t')}\mathrm{d}\omega = 2\pi\delta(t-t'),$$
$$\int_{t_0}^{t} f(t')\delta(t-t')\mathrm{d}t' = \frac{1}{2}f(t), \tag{S.16}$$

we arrive at

$$\frac{\mathrm{d}S}{\mathrm{d}t} = (-i\omega_s - \pi\rho_\omega g_\omega^2)S - i2\pi\rho_\omega g_\omega b_{in}'. \tag{S.17}$$

Eventually, by defining the external coupling rate between the super-atom and channel as $\gamma_{\mathrm{mw},1} = \pi\rho_\omega g_\omega^2$, and the corresponding input fields from the channel $b_{in} = \sqrt{2\pi\rho_\omega} b'_{in}$, obtain the input-output relation in a standard form as

$$\frac{\mathrm{d}S}{\mathrm{d}t} = (-i\omega_s - \gamma_{\mathrm{mw},1})S - i\sqrt{2\gamma_{\mathrm{mw},1}} b_{in}, \tag{S.18}$$

with the transmission

$$b_{out} = b_{in} - i\sqrt{2\gamma_{\mathrm{mw},1}} S. \tag{S.19}$$

At steady state, the super-atom excitation under a microwave signal input at frequency $\omega$ is

$$S(\omega) = \frac{i\sqrt{2\gamma_{\mathrm{mw},1}} b_{in}(\omega)}{-i(\omega_s - \omega) - \gamma_{\mathrm{mw},1}}. \tag{S.20}$$

For one-dimensional contiuous modes with the effect mode area at the cross-section as $A_{\mathrm{eff}}$, we have $\rho_\omega = \frac{1}{2\pi c}$ and $\hbar g_\omega = \sqrt{N} d_{gr} \sqrt{\frac{\hbar\omega}{2\varepsilon_0 A_{\mathrm{eff}}}}$, then we have the coupling rate

$$\gamma_{\mathrm{mw},1} = \pi\rho_\omega g_\omega^2 = \frac{N d_{gr}^2 \omega}{4c\hbar\varepsilon_0 A_{\mathrm{eff}}}. \tag{S.21}$$

Here $d_{gr}$ is the electric dipole moment of the atomic transition $|g\rangle \to |r\rangle$.

### B. Super-atom coupled to multiple channels

The free-space microwave modes can be viewed as the sum of multiple-channel microwave fields. Thus the coupling between the super-atom with the microwave fields in free-space can be described as

$$H = \omega_s S^\dagger S + \sum_{p=1}^{n} \sum_k [\omega_{p,k} b_{p,k}^\dagger b_{p,k} + g_{p,k} b_{p,k}^\dagger S + g_{p,k}^* b_{p,k} S^\dagger]. \tag{S.22}$$

Here the subscript $p$ denotes the $p^{th}$ channel. The evolution equations of operators are

$$\frac{\mathrm{d}b_{p,k}}{\mathrm{d}t} = i[H, b_{p,k}] = -i\omega_{p,k} b_{p,k} - i g_{p,k} S,$$
$$\frac{\mathrm{d}S}{\mathrm{d}t} = i[H, S] \simeq -i\omega_s S - i\sum_{p=1}^{n}\sum_k g_{p,k} b_{p,k}. \tag{S.23}$$

Taking the same method as for single-channel coupling to solve the solution of $S$, we can obtain

$$\frac{\mathrm{d}S}{\mathrm{d}t} = (-i\omega_s - \sum_{p=1}^{n} [\pi\rho_{p,\omega} g_{p,\omega}^2])S - i\sum_{p=1}^{n} [2\pi\rho_{p,\omega} g_{p,\omega} a_{p,in}]$$
$$= (-i\omega_s - \sum_{p=1}^{n} \gamma_p)S - i\sum_{p=1}^{n} \sqrt{2\gamma_p} b_{p,in}. \tag{S.24}$$

Through the Fourier transform, the steady solution of $S$ is

$$S = \frac{-i\sum_{p=1}^{n} \sqrt{2\gamma_p} b_{p,in}(\omega)}{-i(\omega - \omega_s) + \sum_{p=1}^{n} \gamma_p}. \tag{S.25}$$

We can find that the form of this static solution of $S$ is consistent with that of the absorption spectra of a single atom. The coupling rate $\sum_{p=1}^{n} \gamma_p$ between the super-atom with the microwave modes in the total channel, noted as $\gamma_R$, is $N$ times the rate of spontaneous radiation of a single atom $\gamma_{gr}$ in free-space, i.e.

$$\gamma_R = \sum_{p=1}^{n} \gamma_p$$
$$= N\gamma_{gr} = N\frac{\mathrm{d}_{gr}^2 \omega_{gr}^3}{6\pi\hbar\varepsilon_0 c^3}. \tag{S.26}$$

Here $\mathrm{d}_{gr}$ and $\omega_{gr}$ are the electric dipole moment and frequency of the atomic transition $|g\rangle \to |r\rangle$, respectively.

## III. OPTICAL COUPLING

For the coupling between optical fields and atom ensemble, we only consider a simplied two level model, with transition frequency $\omega_{ge}$ and the spontaneous emission rate $\gamma_e$.

### A. The spin-wave mode

The interaction between optical fields and atoms, considering all free-space plane-wave optical modes, can be described by the Hamiltonian:

$$H = \sum_{\vec{k}_0} \sum_{j=1}^{N} g_{j,\vec{k}_0} a_{\vec{k}_0}^\dagger \sigma_{ge,j} e^{i(\omega_{a,\vec{k}_0} - \omega_{ge})t} + h.c., \tag{S.27}$$

where $\vec{k_0}$ is the vector of plane waves and $\sigma_{ge,j}$ is the jump operator for the $j^{th}$ atom, and the summation is over all optical modes and atoms at different locations. Introducing the spin-wave mode of atomic excitation with very low excitation numbers, i.e.,

$$E_{\vec{k}} = \frac{1}{\sqrt{N}} \sum_j e^{i\vec{k}\cdot\vec{r}_j} \sigma_{ge,j} \tag{S.28}$$

$$\sigma_{ge,j} = \frac{1}{\sqrt{N}} \sum_{\vec{k}} e^{-i\vec{k}\cdot\vec{r}_j} E_{\vec{k}}, \tag{S.29}$$

the Hamiltonian can be rewritten in momentum space as

$$H = \frac{|g|}{\sqrt{N}} \sum_{\vec{k}_0} \sum_{\vec{k}_1} \sum_{j=1}^{N} e^{i(\vec{k}_0 - \vec{k}_1)\cdot\vec{r}_j} e^{i(\omega_{a,\vec{k}_0} - \omega_{ge})t} a_{\vec{k}_0}^\dagger E_{\vec{k}_1} + h.c.. \tag{S.30}$$

For a cold atom ensemble with a spatial distribution approximated by Gaussian distributions, we can replace the the summation with the integration of the density function

$$\sum_{j}^{N} = N\int\int\int \rho_{\mathrm{density}} \mathrm{d}x\mathrm{d}y\mathrm{d}z$$
$$= N\int\int\int \frac{1}{\sqrt{2\pi}^3 \sigma_x\sigma_y\sigma_z} e^{\frac{-x^2}{2\sigma_x^2}} e^{\frac{-y^2}{2\sigma_y^2}} e^{\frac{-z^2}{2\sigma_z^2}} \mathrm{d}x\mathrm{d}y\mathrm{d}z. \tag{S.31}$$

The space integral yields

$$\int_{-\infty}^{\infty}\frac{1}{\sqrt{2\pi}\sigma_x}e^{-\frac{x^2}{2\sigma_x^2}}e^{i(k_{0,x}-k_{1,x})x}\mathrm{d}x\simeq e^{-\frac{1}{2}(k_{0,x}-k_{1,x})^2\sigma_x^2}. \quad (S.32)$$

For cold atomic systems with a cigar-shaped spatial distribution, $\sigma_x,\sigma_y\ll\sigma_z$. Thus, for a determined probe light $a_{k_0}$, any spin-wave in the $x$- and $y$-directions can be effectively coupled to that signal light, while only optical spin-waves consistent with the signal light, i.e., $k_{1,z}\simeq k_{0,z}$, can be efficiently excited. It is becuased that $\sigma_x$ and $\sigma_y$ are small enough to satisfy $(k_{0,x}-k_{1,x})^2\sigma_x^2\simeq 0$ and $(k_{0,y}-k_{1,y})^2\sigma_y^2\simeq 0$, and $\sigma_z\gg\sigma_x,\sigma_y$.

Considering only the optical spin-wave mode with vector $\vec{k}_z$, and assuming that the spin-wave modes are not coupled to each other, i.e., each spin-wave mode is considered to be independently coupled to the light-field modes, while the moving and dephasing effects of atoms are neglected. Then, the coupling Hamiltonian in momentum space can be simplified as

$$H=\sqrt{N}|g|\sum_{\vec{k}_0}\sum_{\vec{k}_1}a_{\vec{k}_0}^{\dagger}E_{\vec{k}_1}e^{-\frac{1}{2}[(\vec{k}_0-\vec{k}_1)\vec{\sigma}]^2}e^{i(\omega_{a,\vec{k}_0}-\omega_{ge})t}+h.c. \quad (S.33)$$

In the frame of polar coordinates, we can rewrite

$$\sum_{\vec{k}_0}\rightarrow\sum_{k_0}^{\infty}\sum_{k_{0,z}}^{k_0}\sum_{\theta}, \quad (S.34)$$

where $k_{0,x}$ and $k_{0,y}$ can be presented as

$$\begin{aligned} k_{0,x}=&\sqrt{k_0^2-k_{0,z}^2}\cos\theta,\\ k_{0,y}=&\sqrt{k_0^2-k_{0,z}^2}\sin\theta. \end{aligned} \quad (S.35)$$

For the optical spin-wave with wave vector $\vec{k}_z$, the coupling Hamiltonian between the optical spin-wave $E_{\vec{k}_1}$ with the optical fields can be shown as

$$\begin{aligned} H=&\sqrt{N}|g|\sum_{\vec{k}_0}\left[a_{\vec{k}_0}^{\dagger}E_{\vec{k}_1}e^{-\frac{1}{2}[(\vec{k}_0-\vec{k}_1)\vec{\sigma}]^2}e^{i(\omega_{a,\vec{k}_0}-\omega_{ge})t}+h.c.\right]\\ =&\sqrt{N}|g|\sum_{\theta}\sum_{k_0}^{\infty}\sum_{k_{0,z}}^{k_0}\left[e^{-\frac{1}{2}k_{0,x}^2\sigma^2}e^{-\frac{1}{2}k_{0,y}^2\sigma^2}e^{-\frac{1}{2}(k_{0,z}-k_{1,z})^2\sigma_z^2}\right.\\ &\left.e^{i(k_0-k_{ge})ct}k_0a_{\vec{k}_0}^{\dagger}E_{\vec{k}_1}+h.c.\right]\\ \simeq&A\sqrt{N}|g|\sum_{k_0=-\infty}^{\infty}\left[e^{-\frac{1}{2}(k_0-k_1)^2\sigma_z^2}e^{i(k_0-k_{ge})ct}k_0r_{k_0}^{\dagger}E_{\vec{k}_1}\right.\\ &\left.+h.c.\right], \end{aligned} \quad (S.36)$$

where

$$r_{k_0}^{\dagger}=\frac{1}{A}\sum_{k_{0,z}}^{k_0}\sum_{\theta}e^{-\frac{1}{2}(k_0^2-k_{0,z}^2)\sigma^2}a_{\vec{k}_0}^{\dagger}, \quad (S.37)$$

is a reconstructed bosonic operator of the optical field, whose form is related to the spatial distribution $\rho_{\text{density}}$ of the atomic system and $A$ is the normalization factor. According to commutation relation $[r_{k_0}^{\dagger},r_{k_0}]=-1$, we can get

$$\begin{aligned} &[r_{k_0}^{\dagger},r_{k_0}]\\ =&\frac{1}{|A|^2}\sum_{k_{0,z}}^{k_0}\sum_{\theta}e^{-(k_0^2-k_{0,z}^2)\sigma^2}[a_{\vec{k}_0}^{\dagger},a_{\vec{k}_0}]\\ =&\frac{1}{|A|^2}\int_0^{k_0}\int_0^{2\pi}\rho e^{-(k_0^2-(k_0-\delta)^2)\sigma^2}\mathrm{d}\delta\mathrm{d}\theta\\ \simeq&\frac{1}{|A|^2}\int_0^{k_0}\int_0^{2\pi}\rho e^{-(k_0^2-k_0^2+2k_0\delta)\sigma^2}\mathrm{d}\delta\mathrm{d}\theta\\ =&\frac{1}{|A|^2}2\pi\rho_{2D}\frac{1-e^{-2k_0^2\sigma^2}}{2k_0\sigma^2}\\ \simeq&\frac{1}{|A|^2}\frac{\pi\rho_{2D}}{k_0\sigma^2}\\ =&-1. \end{aligned} \quad (S.38)$$

Thus, we derive the normalization factor as

$$|A|^2\simeq\frac{\pi\rho_{2D}}{k_0\sigma^2}, \quad (S.39)$$

where $\rho_{2D}$ is the optical mode density of two-dimensional free-space, $\delta=k_0-k_{0,z}$, and $\sigma_x=\sigma_y=\sigma$.

### B. The evolution of the system

Based on the effective Hamiltonian derived in the previous section, the evolution of the operators can be described as

$$\begin{aligned} \frac{\mathrm{d}E_{\vec{k}_1}}{\mathrm{d}t}=&-iA\sqrt{N}|g|\sum_{k_0}^{\infty}e^{-\frac{1}{2}(k_0-k_1)^2\sigma_z^2}k_0r_{k_0},\\ \frac{\mathrm{d}r_{k_0}}{\mathrm{d}t}=&-i(k_0-k_{ge})cr_{k_0}\\ &-iA\sqrt{N}|g|e^{-\frac{1}{2}(k_0-k_1)^2\sigma_z^2}k_0E_{\vec{k}_1}. \end{aligned} \quad (S.40)$$

According to the differential equation for $r_{k_0}$, the solution should be of the form

$$r_{k_0}=e^{-i(k_0-k_{ge})ct}f(t). \quad (S.41)$$

Comparing the differentials of this form with the evolution equation for $r_{k_0}$ as

$$\begin{aligned} \frac{\mathrm{d}r_{k_0}}{\mathrm{d}t}=&-i(k_0-k_{ge})cr_{k_0}+e^{-i(k_0-k_{ge})ct}\frac{\mathrm{d}f(t)}{\mathrm{d}t},\\ \frac{\mathrm{d}r_{k_0}}{\mathrm{d}t}=&-i(k_0-k_{ge})cr_{k_0}\\ &-iA\sqrt{N}|g|e^{-\frac{1}{2}(k_0-k_1)^2\sigma_z^2}k_0E_{\vec{k}_1}, \end{aligned} \quad (S.42)$$

we obtain

$$\frac{\mathrm{d}f(t)}{\mathrm{d}t}=-ie^{i(k_0-k_{ge})ct}A\sqrt{N}|g|e^{-\frac{1}{2}(k_0-k_1)^2\sigma_z^2}k_0E_{\vec{k}_1}. \quad (S.43)$$

Integrating this expression from the initial moment $t_0$ gives

$$\begin{aligned} f(t) =& f(t_0) - i\int_{t_0}^{t} e^{i(k_0-k_{ge})ct'} A\sqrt{N}|g| \\ & e^{-\frac{1}{2}(k_0-k_1)^2\sigma_z^2} k_0 E_{\vec{k}_1}(t')\mathrm{d}t'. \end{aligned} \tag{S.44}$$

Substituting this expression back into the solution for $r_{k_0}$, we obtain

$$\begin{aligned} r_{k_0} =& e^{-i(k_0-k_{ge})c(t-t_0)} r_{k_0,\mathrm{in}} - iA\sqrt{N}|g| \\ & e^{-\frac{1}{2}(k_0-k_1)^2\sigma_z^2} \int_{t_0}^{t} e^{-i(k_0-k_{ge})c(t-t')} k_0 E_{\vec{k}_1}(t')\mathrm{d}t', \end{aligned} \tag{S.45}$$

where $r_{k_0,\mathrm{in}} = e^{-i(k_0-k_{ge})ct_0} f(t_0)$ denotes the optical field input at the initial moment $t_0$. Substituting the solution into the evolution equation of the optical spin-wave operator, we can obtain

$$\begin{aligned} \frac{\mathrm{d}E_{\vec{k}_1}}{\mathrm{d}t} =& -iA\sqrt{N}|g| \int_{-\infty}^{\infty} \rho_{1D} e^{-\frac{1}{2}(k_0-k_1)^2\sigma_z^2} e^{-i(k_0-k_{ge})c(t-t_0)} \\ & k_0 r_{k_0,\mathrm{in}} \mathrm{d}k_0 - A^2 N|g|^2 \int_{-\infty}^{\infty} \rho_{1D} e^{-(k_0-k_1)^2\sigma_z^2} \\ & \int_{t_0}^{t} e^{-i(k_0-k_{ge})c(t-t')} k_0 E_{\vec{k}_1}(t')\mathrm{d}t'\mathrm{d}k_0, \end{aligned} \tag{S.46}$$

where the summation over $k_0$ has been replaced by the integral

$$\sum_{k_0=-\infty}^{\infty} \rightarrow \int_{-\infty}^{\infty} \rho_{1D}\mathrm{d}k_0, \tag{S.47}$$

with $\rho_{1D}$ being the optical mode density of two-dimensional free-space. The mode density of the one-dimensional free-space $\rho_{1D}$ is related to the mode density of the two-dimensional free-space $\rho_{2D}$ by:

$$\rho_{1D}\rho_{2D} = 2\frac{L_x L_y L_z}{(2\pi)^3 c}, \tag{S.48}$$

where the factor of 2 accounts for the two polarizations, and $L_{x,y,z}$ are the box quantization lengths in the $x, y$, and $z$ directions, respectively.

Similar to treatment based on Weisskopf-Wigner approximation [1], the coupling terms are insensitive to $k_0$ for $k_0 \approx k_{ge}$. We can therefore replace $k_0$ with $k_{ge}$ in Eq. (S.46), simplifying the integral over $k_0$ as

$$\int_{-\infty}^{\infty} e^{-i(k_0-k_{eg})c(t-t')}\mathrm{d}k_0 = 2\pi\delta(t-t'). \tag{S.49}$$

Applying the following equality of the integral over $t$

$$\int_{t_0}^{t} f(t')\delta(t-t')\mathrm{d}t' = \int_{t}^{t_I} f(t')\delta(t-t')\mathrm{d}t' = \frac{1}{2}f(t), \tag{S.50}$$

we obtain the following evolution equation as

$$\frac{\mathrm{d}E_{\vec{k}_1}}{\mathrm{d}t} = -i\sqrt{N}gA_{\mathrm{in}}(t) - \kappa_{\mathrm{opt},1}E_{\vec{k}_1}(t). \tag{S.51}$$

Here, $A_{\mathrm{in}}(t)$ is a reconstructed annihilation operator of the input optical field, whose form is related to the spatial distribution $\rho_{\mathrm{density}}$ of the atomic system, noted as

$$\begin{aligned} A_{\mathrm{in}}(t) =& A\int_{-\infty}^{\infty} \rho_{1D,\omega} e^{-\frac{1}{2}(k_0-k_1)^2\sigma_z^2} \times \\ & e^{-i(k_0-k_{ge})c(t-t_0)} k_0 r_{k_0,\mathrm{in}} \mathrm{d}k_0, \end{aligned} \tag{S.52}$$

and

$$\begin{aligned} \kappa_{\mathrm{opt},1} =& e^{-(k_{ge}-k_1)^2\sigma_z^2} \pi\rho_{1D} N g_\omega^2 |A|^2 k_{ge} \\ =& e^{-(k_{ge}-k_1)^2\sigma_z^2} \pi 2\frac{L_x L_y L_z}{8\pi^3 c} N d_{ge}^2 \frac{\omega}{4\hbar\varepsilon_0 L_x L_y L_z}\frac{\pi}{\sigma^2} \\ \simeq& e^{-(k_{ge}-k_1)^2\sigma_z^2} \frac{N d_{ge}^2 \omega_{ge}}{16\pi\hbar\varepsilon_0 c\sigma^2}. \end{aligned} \tag{S.53}$$

represents the decay rate of $E_{\vec{k}_1}$.

### C. The mean optical depth $\overline{OD}$

The atomic number is directly related to the optical depth of the atomic system. The mean optical depth $\overline{OD}$ of the atomic system in the direction of optical light propagation is calculated as [2]

$$\begin{aligned} \overline{\mathrm{OD}} =& \frac{\int_{-\infty}^{\infty}\int_{-\infty}^{\infty} e^{\frac{-x^2}{2\sigma_x^2}} e^{\frac{-y^2}{2\sigma_y^2}} \mathrm{d}x\mathrm{d}y \int_{-\infty}^{\infty} N\rho_{\mathrm{density}}\mathrm{d}z\sigma_{\mathrm{scr}}}{\int_{-\infty}^{\infty}\int_{-\infty}^{\infty} e^{\frac{-x^2}{2\sigma_x^2}} e^{\frac{-y^2}{2\sigma_y^2}} \mathrm{d}x\mathrm{d}y} \\ =& \frac{\int_{-\infty}^{\infty}\int_{-\infty}^{\infty} e^{\frac{-x^2}{\sigma_x^2}} e^{\frac{-y^2}{\sigma_y^2}} \mathrm{d}x\mathrm{d}y \int_{-\infty}^{\infty} \frac{N}{\sqrt{2\pi}^3\sigma_x\sigma_y\sigma_z} e^{\frac{-z^2}{2\sigma_z^2}} \mathrm{d}z\sigma_{\mathrm{scr}}}{\int_{-\infty}^{\infty}\int_{-\infty}^{\infty} e^{\frac{-x^2}{2\sigma_x^2}} e^{\frac{-y^2}{2\sigma_y^2}} \mathrm{d}x\mathrm{d}y} \\ =& \frac{\pi\sigma_x\sigma_y \frac{N}{2\pi\sigma_x\sigma_y}\sigma_{\mathrm{scr}}}{2\pi\sigma_x\sigma_y} \\ =& \frac{N\sigma_{\mathrm{scr}}}{4\pi\sigma_x\sigma_y}, \end{aligned} \tag{S.54}$$

where $\sigma_{\mathrm{scr}} = 3\lambda_{ge}^2/(2\pi)$ is the optical absorption cross-section. According to this equation, we can express the atomic number in the ensemble as

$$N = \frac{4\pi\sigma_x\sigma_y\overline{\mathrm{OD}}}{\sigma_{\mathrm{scr}}} = \frac{4\pi\sigma^2\overline{\mathrm{OD}}}{\sigma_{\mathrm{scr}}}. \tag{S.55}$$

Substituting this expression into the Eq. (S.53), which describes the decay rate of the optical spin-wave mode, we obtain

$$\begin{aligned} \frac{\kappa_{\mathrm{opt},1}}{\gamma_e} =& \frac{3}{8\sigma^2}\frac{4\pi\sigma^2\overline{\mathrm{OD}}}{\sigma_{\mathrm{scr}}}\left(\frac{\lambda_{ge}}{2\pi}\right)^2 \\ =& \frac{\overline{\mathrm{OD}}}{4}, \end{aligned} \tag{S.56}$$

where $\gamma_e = \mathrm{d}_{ge}^2\omega_{ge}^3/6\pi\hbar\varepsilon_0 c^3$ is the amplitude decay rate of the excited state $|r\rangle$ of a single atom.

## IV. EFFECTIVE CONVERSION HAMILTONIAN

The original Hamiltonian is

$$H=\sum_{j,k_a,k_b}\omega_s\sigma_{rr}^j+\omega_e\sigma_{ee}^j+\omega_a a_k^\dagger a_k+\omega_b b_k^\dagger b_k+ \left(g_a\sigma_{ge}^j a_k^\dagger+g_b\sigma_{gr}^j b_k^\dagger+\Omega_c\sigma_{re}^j e^{i\omega_c t}+h.c.\right). \quad (S.57)$$

With the rotating frame of $H_0=\omega_a a_k^\dagger a_k+\omega_b b_k^\dagger b_k+\omega_a\sigma_{ee}+\omega_b\sigma_{rr}$, the Hamiltonian can be shown as

$$H=\sum_{j,k_a,k_b}\delta\sigma_{ee}^j+\left(g_a\sigma_{ge}^j a_k^\dagger+g_b\sigma_{gr}^j b_k^\dagger+\Omega_c\sigma_{re}^j+h.c.\right). \quad (S.58)$$

Here, we take $\omega_b=\omega_s$, $\omega_a=\omega_b+\omega_c$ and $\delta=\omega_e-\omega_a$. The above Hamiltonian consists of four parts, the part of eigen energy $\sum_j\sigma_{ee}^j$, the part of optical coupling $\sum_{j,k_a}g_a\sigma_{ge}^j a_k^\dagger$, the part of microwave coupling $\sum_{j,k_b}g_b\sigma_{gr}^j b_k^\dagger$ and the part of driving coupling $\sum_j\Omega_c\sigma_{re}^j$. Using the operators of the super-atom transition $S^\dagger,S$ and the optical spin-wave $E^\dagger,E$, the Hamiltonian can be represented.

With the relation between atomic transition operators and optical spin-wave operators, we can get

$$\begin{aligned}\sum_j\delta\sigma_{ee}^j=&\sum_j\delta\sigma_{eg}^j\cdot\sigma_{ge}^j\\ =&\sum_j\delta\frac{1}{\sqrt{N}}\sum_{\vec{k}_1}e^{i\vec{k}_1\vec{r}_j}E_{\vec{k}_1}^\dagger\cdot\frac{1}{\sqrt{N}}\sum_{\vec{k}_2}e^{-i\vec{k}_2\vec{r}_j}E_{\vec{k}_2}\\ =&\delta\int\rho_{\text{density}}d\vec{r}\sum_{\vec{k}_1,\vec{k}_2}e^{i(\vec{k}_1-\vec{k}_2)\vec{r}_j}E_{\vec{k}_1}^\dagger E_{\vec{k}_2}\\ \simeq&\delta\sum_k E_k^\dagger E_k. \end{aligned}\quad (S.59)$$

Here, considering the fact that the size of atomic space distribution is much larger than the optical wavelength, we can assume that $\vec{k}_1\simeq\vec{k}_2$.

The part of the optical coupling can be represented by replacing atomic operators with optical spin-wave operators, which is the same as Eq. (2) in the main text. The coupling optical modes $a$ can be divided into two parts for analysis, one of which can be collected and excited while the other is not. The coupling of uncollectible modes with optical spin-wave leads to spin-wave loss, as Eq. (S.51). Thus the coupling of all optical modes and optical spin-wave in free-space can be expressed in a simplified way as

$$\begin{aligned}\sum_{j,\vec{k}_a}g_a\sigma_{ge}^j a_k^\dagger=&\frac{|g|}{\sqrt{N}}\sum_{\vec{k}_a}\sum_{\vec{k}_1}\sum_{j=1}^N e^{i(\vec{k}_a-\vec{k}_1)\cdot\vec{r}_j}a_{\vec{k}_a}^\dagger E_{\vec{k}_1}\\ \simeq&\sum_{k_1}g_{a,eff}a_{in}^\dagger E_{k_1}-i\kappa_{\text{opt},1}E_{k_1}^\dagger E_{k_1}.\end{aligned}\quad (S.60)$$

Here the coupling rate of the input optical modes satisfies $g_{a,eff}\le\sqrt{2\kappa_{\text{opt},1}}$. To obtain the optimal conversion efficiency, the ideal $g_{a,eff}\simeq\sqrt{2\kappa_{\text{opt},1}}$ is adopted.

For the part of the microwave coupling, with the definition of $|G\rangle=|g_{\otimes N}\rangle$, $|R\rangle=\frac{1}{\sqrt{N}}\sum_j|gg...r_j...gg\rangle$, $S=|G\rangle\langle R|$ and Eq. (S.24), we can obtain

$$\begin{aligned}\sum_{j,k_b}g_b\sigma_{gr}^j b_k^\dagger=&\sum_k\sqrt{N}g_b|G\rangle\langle R|b_k^\dagger\\ =&\sum_{p=1}^n\sqrt{2\gamma_p}b_{p,in}^\dagger S-i\sum_{p=1}^n\gamma_p S^\dagger S.\end{aligned}\quad (S.61)$$

When the input microwave field as one-dimensional continuous modes, we can obtain

$$\sum_{j,k_b}g_b\sigma_{gr}^j b_k^\dagger=\sqrt{2\gamma_{\text{mw},1}}b_{in}^\dagger S-i\sum_{p=1}^n\gamma_p S^\dagger S. \quad (S.62)$$

Considering the case where only one atom can be excited to an excited state and the Rabi frequency $\Omega_c$ of the control field is much larger than the decay rate $\gamma_e$ of the excite state $|e\rangle$ ($\Omega_c\gg\gamma_e$) [3, 4], with the definition of $S^\dagger=|R\rangle\langle G|$ and the relation between $\sigma_{eg}$ and optical spin-wave $E$ ($\sigma_{ge,j}=\frac{1}{\sqrt{N}}\sum_{\vec{k}}e^{-i\vec{k}\cdot\vec{r}_j}E_{\vec{k}}$), we can obtain

$$\begin{aligned}\sum_j\Omega_c e^{ik_c r_j}\sigma_{re}^j=&\sum_j\Omega_c e^{ik_c r_j}\sigma_{rg}^j\sigma_{ge}^j\\ =&\sqrt{N}\Omega_c S^\dagger\frac{1}{\sqrt{N}}\sum_k e^{-i(k-k_c)r_j}E_k\\ \simeq&\sum_k\Omega_c S^\dagger E_k.\end{aligned}\quad (S.63)$$

with approximation $|G\rangle\langle G|=I$. Here we also take the approximation that $e^{-i(k-k_c)r_j}\simeq 1$ for small atomic size and small difference between $k_c$ and $k$.

Given the optical spin-waves $\sum_k E_k$ are independently coupled to the optical fields, the original Hamiltonian Eq. (S.58) can be rewritten as

$$\begin{aligned}H=&\delta E^\dagger E+(\sqrt{2\kappa_{\text{opt},1}}a_{in}^\dagger E+\sqrt{2\gamma_{\text{mw},1}}b_{in}^\dagger S+\\ &\Omega_c S^\dagger E+h.c.),\end{aligned}\quad (S.64)$$

which is the same as Eq. (3) in the main text.

## V. METHOD OF SLICING

In the main text, we only consider the model with the length of the atom cloud much smaller than the wavelength of microwave. However, in practical experiments, it is potential to realize a much longer atom cloud by weakening the confinement of magneto-optics trap in $z$-direction [5, 6]. Here, we show that such a situation can also be approximately solved with our model by the method of "slicing", i.e., treat the long atom cloud as a chain of many short slices with each slice could be treated as a single super-atom. Therefore, the MOC of the entire atom cloud can be obtained by solving cascaded

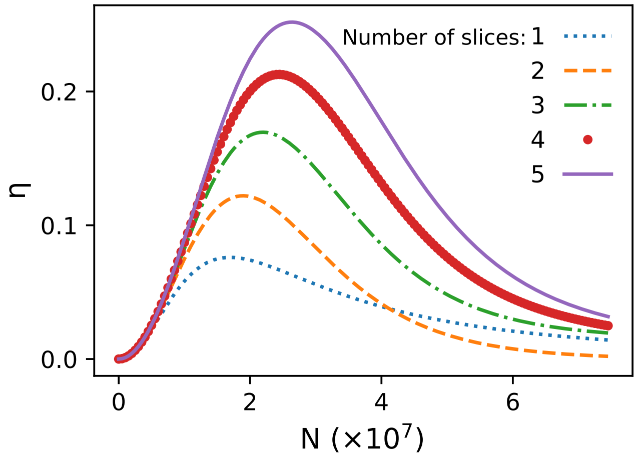


**Supplemental Figure** 3. The dependence of conversion efficiency $\eta$ on the total atom number $N$ for various atom ensemble slices, with each slice has a length of $\lambda_{\mathrm{m}}/2$, with the parameters are the same as the main text.

slices. For each slice, the MOC can be represented by a transfer matrix $\mathbf{T}$ for the forwardly propagating optical and microwave modes, i.e.

$$\begin{pmatrix} a_{\mathrm{out}} \\ b_{\mathrm{out}} \end{pmatrix} = \mathbf{T} \begin{pmatrix} a_{\mathrm{in}} \\ b_{\mathrm{in}} \end{pmatrix}. \tag{S.65}$$

According to the input-output relationships

$$\begin{aligned} a_{\mathrm{out}} &= a_{\mathrm{in}} - i\sqrt{2\kappa_{\mathrm{opt},1}}E, \\ b_{\mathrm{out}} &= b_{\mathrm{in}} - i\sqrt{2\gamma_{\mathrm{mw},1}}S, \end{aligned} \tag{S.66}$$

we obtain the elements of the transfer matrix as

$$\mathbf{T} = \begin{pmatrix} \frac{i\delta/\kappa_{\mathrm{opt},1}+C-1}{i\delta/\kappa_{\mathrm{opt},1}+C+1} & \frac{\frac{i2\Omega_c}{\gamma_{\mathrm{R}}}\sqrt{\frac{\gamma_{\mathrm{mw},1}}{\kappa_{\mathrm{opt},1}}}}{i\delta/\kappa_{\mathrm{opt},1}+C+1} \\ \frac{\frac{i2\Omega_c}{\gamma_{\mathrm{R}}}\sqrt{\frac{\gamma_{\mathrm{mw},1}}{\kappa_{\mathrm{opt},1}}}}{i\delta/\kappa_{\mathrm{opt},1}+C+1} & \frac{-i2\frac{\delta\gamma_{\mathrm{mw},1}}{\kappa_{\mathrm{opt},1}\gamma_{\mathrm{R}}}-2\frac{\gamma_{\mathrm{mw},1}}{\gamma_{\mathrm{R}}}+i\frac{\delta}{\kappa_{\mathrm{opt},1}}+C+1}{i\delta/\kappa_{\mathrm{opt},1}+C+1} \end{pmatrix}. \tag{S.67}$$

When the atomic ensemble is divided into $n$ slices, the final output should be obtained as

$$\begin{pmatrix} a_{\mathrm{out}} \\ b_{\mathrm{out}} \end{pmatrix} = \mathbf{T}^n \begin{pmatrix} a_{\mathrm{in}} \\ b_{\mathrm{in}} \end{pmatrix}. \tag{S.68}$$

Thus the conversion efficiency from microwave to optical frequency is $\eta = |\mathbf{T}^n[0,1]|^2$.

Taking the same parameters as Fig. 4 in the main text, the conversion efficiency for different number of slices is calculated and the result is shown as Supplemental Figure 3 Here, we define the length of each slice as $\lambda_{\mathrm{m}}/2$, within which the microwave transitions of atoms approximately has a uniform coupling strength and phase to all free-space microwave mode, and a total atom of $N$ atoms are equally divided into each slices. The results indicate that when the number of atoms are smaller than $7\times10^6$, the conversion efficiency $\eta$ is insensitive to the length of the atom cloud $L = n\lambda_{\mathrm{m}}/2$. However, when the atom number is larger, $\eta$ can be improved by increasing the length of atom ensemble while $\eta$ for a single super-atom is limited due to $C > 1$. We find that the dependence of $\eta$ on $N$ for different slice number $n$ show similar behaviors, as there is an optimal $N$. For the experimental situation in Ref. [6], where the length of the atomic ensemble is $L = 21\,\mathrm{mm}$, the highest achieved $\eta$ can be improved to 25% as $n \approx 5$ for $\lambda_m = 8$ mm.


* zyl12@ustc.edu.cn
† clzou321@ustc.edu.cn



[1] D. Wall and G. Milburn, *Quantum Optics* (Springer Berlin Heidelberg, Berlin, Heidelberg, 2008).
[2] B. Zhu, J. Cooper, J. Ye, and A. M. Rey, Light scattering from dense cold atomic media, Physical Review A **94**, 023612 (2016).
[3] E. Brion, L. H. Pedersen, and K. Mølmer, Adiabatic elimination in a lambda system, Journal of Physics A: Mathematical and Theoretical **40**, 1033 (2007).
[4] V. Paulisch, H. Rui, H. K. Ng, and B.-G. Englert, Beyond adiabatic elimination: A hierarchy of approximations for multi-photon processes, The European Physical Journal Plus **129**, 12 (2014).
[5] Y. Wang, J. Li, S. Zhang, K. Su, Y. Zhou, K. Liao, S. Du, H. Yan, and S.-L. Zhu, Efficient quantum memory for single-photon polarization qubits, Nature Photonics **13**, 346 (2019).
[6] H.-T. Tu, K.-Y. Liao, Z.-X. Zhang, X.-H. Liu, S.-Y. Zheng, S.-Z. Yang, X.-D. Zhang, H. Yan, and S.-L. Zhu, High-efficiency coherent microwave-to-optics conversion via off-resonant scattering, Nature Photonics **16**, 291 (2022).
